# Supplementary material for: FSPGD: Rethinking Black-box Attacks on Semantic Segmentation
Source: arXiv:2502.01262 source file (2026-09-04)
Supplement: Supplementary file 1 [file X_suppl.tex]

% \clearpage
% \setcounter{page}{1}
% \maketitlesupplementary

% \section{Rationale}
% \label{sec:rationale}
% % 
% Having the supplementary compiled together with the main paper means that:
% % 
% \begin{itemize}
% \item The supplementary can back-reference sections of the main paper, for example, we can refer to \cref{sec:intro};
% \item The main paper can forward reference sub-sections within the supplementary explicitly (e.g. referring to a particular experiment); 
% \item When submitted to arXiv, the supplementary will already included at the end of the paper.
% \end{itemize}
% % 
% To split the supplementary pages from the main paper, you can use \href{https://support.apple.com/en-ca/guide/preview/prvw11793/mac#:~:text=Delete%20a%20page%20from%20a,or%20choose%20Edit%20%3E%20Delete).}{Preview (on macOS)}, \href{https://www.adobe.com/acrobat/how-to/delete-pages-from-pdf.html#:~:text=Choose%20%E2%80%9CTools%E2%80%9D%20%3E%20%E2%80%9COrganize,or%20pages%20from%20the%20file.}{Adobe Acrobat} (on all OSs), as well as \href{https://superuser.com/questions/517986/is-it-possible-to-delete-some-pages-of-a-pdf-document}{command line tools}.
\maketitlesupplementary

\setcounter{page}{1}

% -----------------------------------------------------------------------
\setcounter{section}{0} % add yg
\setcounter{figure}{0}  % add yg
\setcounter{table}{0}  % add yg

\section{Visualization of Feature Similarity}
To further validate the motivation described in Sec.~\ref{sec3.1.motivation} , we performed visualizations on a broader variety of images. Figs.~\ref{sup_fig:figs1} and ~\ref{sup_fig:figs2} present experimental results on the Pascal VOC 2012 dataset, while Figs.~\ref{sup_fig:figs3} and Figs.~\ref{sup_fig:figs4} show results on the Cityscapes dataset. As seen in the figures, conventional methods maintain the similarity of features within the same class even after performing an attack, leading to poor attack performance on new target models. In contrast, the proposed method reduces feature similarity and exhibits superior attack performance compared to conventional methods.

\begin{figure}[htbp]
\centering
\includegraphics[width=0.98\linewidth]{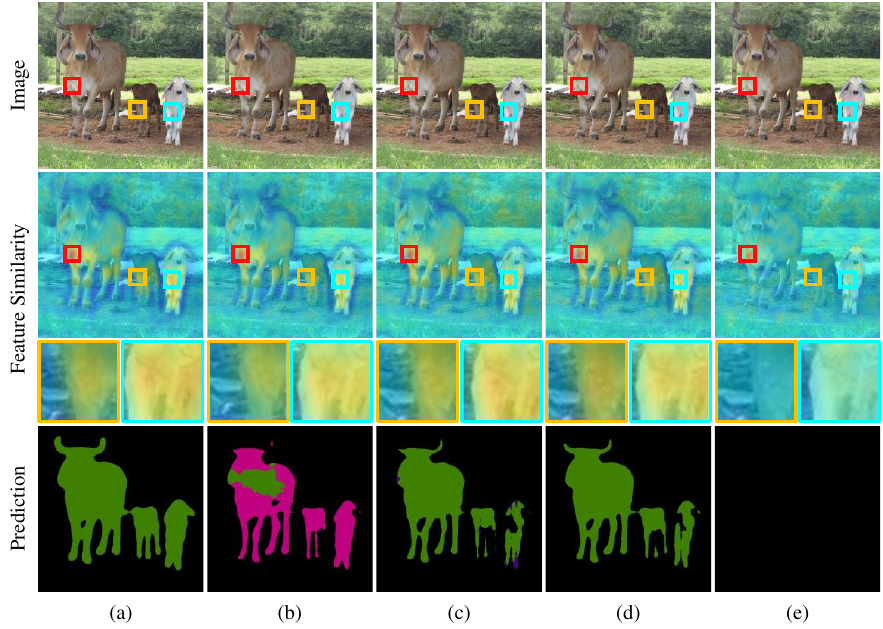}
\caption{Visualization of the feature similarity on Pascal VOC 2012 dataset. Red boxes indicate the reference features, while yellow and blue boxes represent regions belonging to the same class as the red boxes. Deeplabv3-Res50 is used as the source model and Deeplabv3-Res101 is used as target model. (a) Clean image, (b) PGD~\cite{mkadry2017towards}, (c) SegPGD~\cite{gu2022segpgd}, (d) CosPGD~\cite{agnihotri2024cospgd}, (e) FSPGD (Ours).}
\label{sup_fig:figs1}
\end{figure}

\begin{figure}[htbp]
\centering
\includegraphics[width=0.98\linewidth]{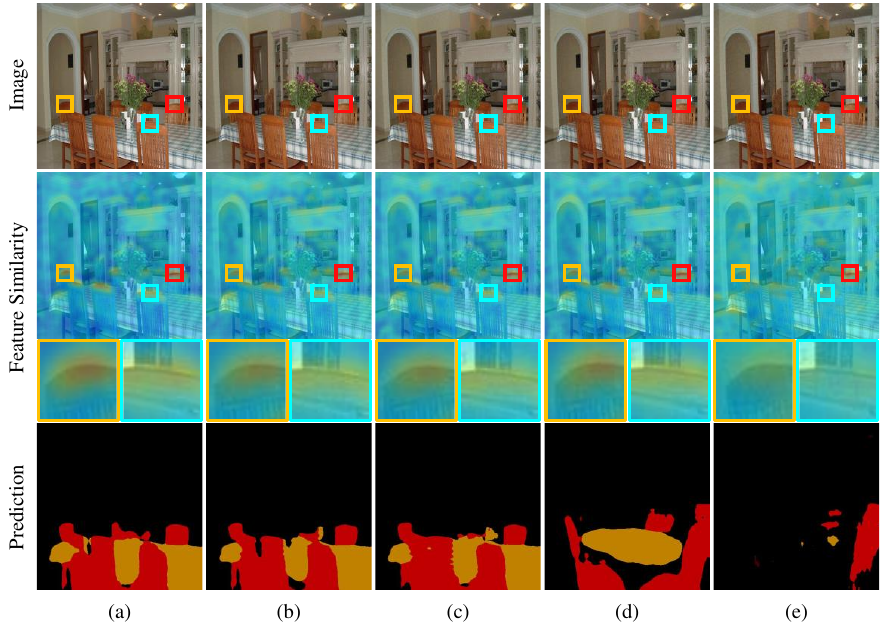}
\caption{Visualization of the feature similarity on Pascal VOC 2012 dataset. Red boxes indicate the reference features, while yellow and blue boxes represent regions belonging to the same class as the red boxes. Deeplabv3-Res50 is used as the source model and Deeplabv3-Res101 is used as target model. (a) Clean image, (b) PGD~\cite{mkadry2017towards}, (c) SegPGD~\cite{gu2022segpgd}, (d) CosPGD~\cite{agnihotri2024cospgd}, (e) FSPGD (Ours).}
\label{sup_fig:figs2}
\end{figure}

% \begin{figure}[h]
% \centering
% \includegraphics[width=0.98\linewidth]{supple_similarity_city1.pdf}
% \caption{Visualization of the feature similarity on Cityscapes dataset. Red boxes indicate the reference features, while yellow and blue boxes represent regions belonging to the same class as the red boxes. Deeplabv3-Res50 is used as the source model and Deeplabv3-Res101 is used as target model. (a) Clean image, (b) PGD~\cite{mkadry2017towards}, (c) SegPGD~\cite{gu2022segpgd}, (d) CosPGD~\cite{agnihotri2024cospgd}, (e) FSPGD (Ours).}
% \label{sup_fig:figs3}
% \end{figure}

\begin{figure}[htbp]
\centering
\includegraphics[width=0.9\linewidth]{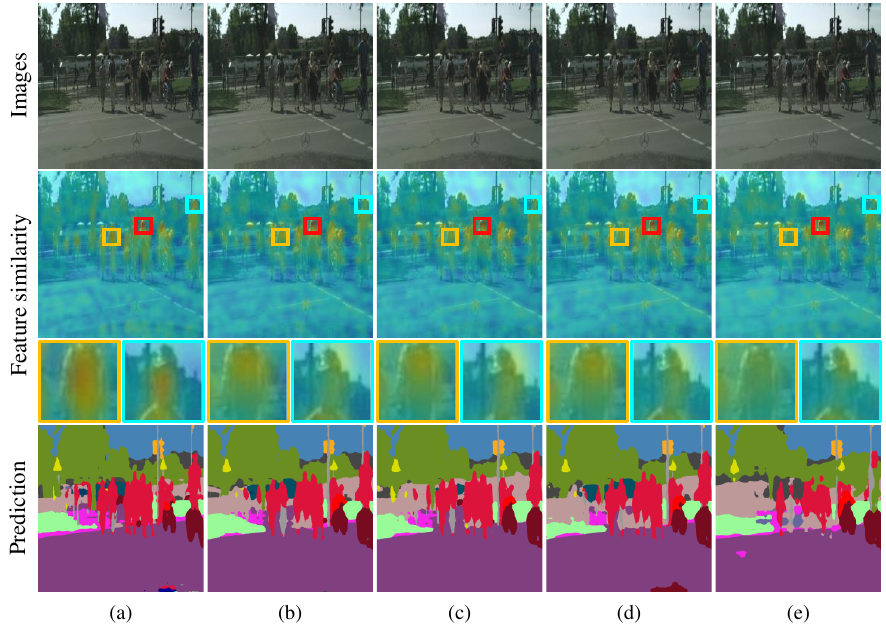}
\caption{Visualization of the feature similarity on Cityscapes dataset. Red boxes indicate the reference features, while yellow and blue boxes represent regions belonging to the same class as the red boxes. Deeplabv3-Res50 is used as the source model and Deeplabv3-Res101 is used as target model. (a) Clean image, (b) PGD~\cite{mkadry2017towards}, (c) SegPGD~\cite{gu2022segpgd}, (d) CosPGD~\cite{agnihotri2024cospgd}, (e) FSPGD (Ours).}
\label{sup_fig:figs3}
\end{figure}

\begin{figure}[htbp]
\centering
\includegraphics[width=0.9\linewidth]{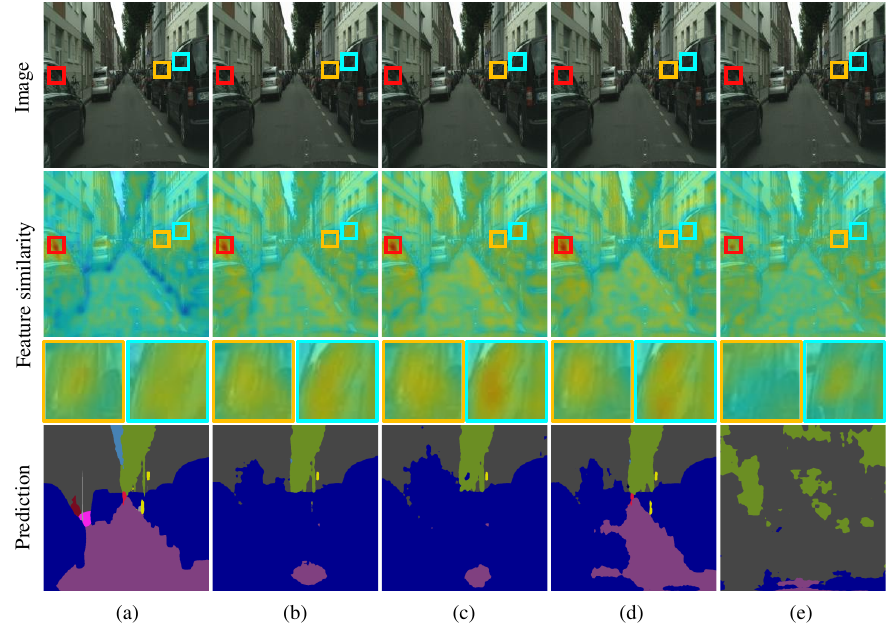}
\caption{Visualization of the feature similarity on Cityscapes dataset. Red boxes indicate the reference features, while yellow and blue boxes represent regions belonging to the same class as the red boxes. Deeplabv3-Res50 is used as the source model and Deeplabv3-Res101 is used as target model. (a) Clean image, (b) PGD~\cite{mkadry2017towards}, (c) SegPGD~\cite{gu2022segpgd}, (d) CosPGD~\cite{agnihotri2024cospgd}, (e) FSPGD (Ours).}
\label{sup_fig:figs4}
\end{figure}

\FloatBarrier
\newpage

% -----------------------------------------------------------------------

\section{Extended Experimental Results}
\label{sec: B}
To further prove the superiority of the proposed method, we conducted comparative experiments with various conventional methods~\cite{mkadry2017towards, gu2022segpgd, agnihotri2024cospgd, xie2017adversarial, lin2019nesterov, xie2019improving, dong2019evading}. To evaluate the transferability of the attack methods, we designed the experiments with non-overlapping encoders for the source model and target model. As shown in Table~\ref{sup_table1} and ~\ref{sup_table2}, the proposed method achieves the best performance among black-box attack methods on the source model (CosPGD~\cite{agnihotri2024cospgd} is a white-box attack method) and shows superior attack performance on target models compared to existing methods.

% ----------------------PASCAL VOC 2012---------------------------------------

\begin{table}[htbp]
\caption{Attack performance comparison on Pascal VOC 2012 in terms of mIoU. Lower mIoU means better performance and bold numbers denote the best mIoU values for each experimental setup}
\begin{center}
\setlength{\tabcolsep}{10pt}
\begin{tabular}{c | c | c  c  c  c}
\Xhline{3\arrayrulewidth}
& & \multicolumn{4}{c}{Target Models (mIoU$\downarrow$)} \\
\hline
\multirow{2}*{Source Models} & Attack Method & Source Model & PSPRes101 & DV3Res101 & FCNVGG16\\
\cline{2-6}
& Clean Images & 80.22/80.18 & 78.39 & 82.88 & 59.80 \\
\hline
\multirow{8}*{PSPRes50} & PGD~\cite{mkadry2017towards} & 7.72 & 54.73& 59.41     & 45.70  \\
& SegPGD~\cite{gu2022segpgd}& 5.41  & 54.10  & 58.95    & 45.43  \\
& CosPGD~\cite{agnihotri2024cospgd} &1.84   & 56.63 & 64.37    & 45.99   \\
& DAG~\cite{xie2017adversarial}& 65.82  & 62.67 & 66.22& 38.91         \\
& NI~\cite{lin2019nesterov}&  7.71 & 33.49   & 38.52   & 32.94  \\
& DI~\cite{xie2019improving} & 6.41& 32.00 & 35.25   & 37.34    \\
& TI~\cite{dong2019evading} & 18.28 & 64.50 & 69.60& 36.80  \\
& FSPGD (Ours) &  3.39 & \textbf{22.24} & \textbf{16.84} & \textbf{19.75} \\

\hline
\multirow{8}*{DV3Res50} & PGD~\cite{mkadry2017towards}& 9.74 & 52.96 &  56.35 & 46.39 \\
& SegPGD~\cite{gu2022segpgd} & 7.26 &52.05 & 56.50 & 46.23 \\
& CosPGD~\cite{agnihotri2024cospgd} &\textbf{1.67} & 56.82 &  61.36 & 45.94 \\
& DAG~\cite{xie2017adversarial} & 66.78 & 62.12 & 66.84 & 38.77 \\
& NI~\cite{lin2019nesterov}& 9.89 & 33.86 &36.85 & 34.92 \\
& DI~\cite{xie2019improving} & 7.35 &31.93 & 32.93 &38.30 \\
& TI~\cite{dong2019evading}  & 19.34 &64.99 & 69.80 & 37.65 \\
& FSPGD(Ours) & 3.44 & \textbf{21.89} & \textbf{16.57} & \textbf{19.36} \\
\hline
\hline
\multirow{2}*{Source Models} & Attack Method & Source Model & PSPRes50 & DV3Res50 & FCNVGG16\\
\cline{2-6}
& Clean Images & 78.39/82.88  & 80.22 & 80.18 & 59.80 \\ 
\hline
\multirow{8}*{PSPRes101}& PGD~\cite{mkadry2017towards} &10.13 & 55.39 &  55.39 &  47.25 \\
& SegPGD~\cite{gu2022segpgd} & 7.31 & 53.56 & 54.03  & 46.26 \\
& CosPGD~\cite{agnihotri2024cospgd} &\textbf{2.87} & 57.74  &  58.50  & 47.05 \\
& DAG~\cite{xie2017adversarial} & 63.36 & 66.28  & 66.06  & 39.10 \\
& NI~\cite{lin2019nesterov} & 10.22& 33.50   & 34.12  & 34.41 \\
& DI~\cite{xie2019improving} &7.21 &  29.00  & 30.58 & 39.24 \\
& TI~\cite{dong2019evading} &22.23 & 64.64  &  64.95 &  37.29 \\
& FSPGD(Ours) &  2.99 & \textbf{12.48} & \textbf{13.54} & \textbf{21.30} \\
\hline
\multirow{8}*{DV3Res101}& PGD~\cite{mkadry2017towards} & 9.75 & 59.36 & 55.54 & 47.48 \\
& SegPGD~\cite{gu2022segpgd} & 7.18 &54.47  & 53.96 & 46.53 \\
& CosPGD~\cite{agnihotri2024cospgd} & \textbf{2.73} &58.83  & 58.54 & 47.25 \\
& DAG~\cite{xie2017adversarial} & 67.55 & 67.09 & 67.58 & 39.48 \\
& NI~\cite{lin2019nesterov} &  9.49  &36.41 & 34.75 & 35.62 \\
& DI~\cite{xie2019improving} & 7.64  &34.87 & 34.11 &  40.99 \\
& TI~\cite{dong2019evading} & 27.16  & 65.79 & 65.13 & 37.98 \\
& FSPGD(Ours) &3.28 & \textbf{11.42} & \textbf{13.45} & \textbf{21.49} \\
\Xhline{3\arrayrulewidth}
\end{tabular}
\end{center}
\label{sup_table1}
\end{table}

% ----------------------Cityscapes RESNET---------------------------------------

\begin{table}[htbp]
\caption{Attack performance comparison on Cityscapes in terms of mIoU. Lower mIoU means better performance and bold numbers denote the best mIoU values for each experimental setup}
\begin{center}
\begin{tabularx}{\textwidth}{c|c|>{\centering\arraybackslash}X >{\centering\arraybackslash}X >{\centering\arraybackslash}X >{\centering\arraybackslash}X >{\centering\arraybackslash}X}
\Xhline{3\arrayrulewidth}
& & \multicolumn{5}{c}{Target Models (mIoU$\downarrow$)}\\
\hline
\multirow{3}*{Source Models} & \multirow{2}*{Attack Method} & Source & PSP & DV3 & Segformer & Maskformer \\
& & Model & Res101 & Res101 & MiT-B0 & Swin-S \\
\cline{2-7}
& Clean Images & 64.62 / 65.90 &65.65 &67.16 & 60.58 & 68.24\\
\hline
\multirow{7}*{PSP} & PGD~\cite{mkadry2017towards}& 1.83  & 18.80 & 19.35 & 48.92 & 59.66 \\
\multirow{7}*{Res50} & SegPGD~\cite{gu2022segpgd}& 1.38  & 18.26 & 19.34 & 49.83 & 60.41 \\
& CosPGD~\cite{agnihotri2024cospgd} & \textbf{0.07}  & 24.90 & 26.65 & 50.31 & 60.53 \\
& DAG~\cite{xie2017adversarial} &23.52 & 36.76 & 33.47 & 50.24 & 60.64 \\
& NI~\cite{lin2019nesterov}&  1.62  & 15.07 & 17.07 & 44.43 & 50.09 \\
& DI~\cite{xie2019improving}&  1.92  & 17.60 & 21.57 & 52.12 & 54.81 \\
& TI~\cite{dong2019evading} &1.64  & 28.39 & 34.07 & 51.91 & 58.70 \\
& FSPGD (Ours) &0.93  &\textbf{ 5.12}  & \textbf{3.29}  & \textbf{41.30} & \textbf{47.30} \\
\hline
\multirow{7}*{DV3} & PGD~\cite{mkadry2017towards}&  2.00  & 22.19 & 22.06 & 50.28 & 60.64 \\
\multirow{7}*{Res50} & SegPGD~\cite{gu2022segpgd} & 0.96  & 22.20 & 22.51 & 50.59 & 60.24 \\
& CosPGD~\cite{agnihotri2024cospgd} & \textbf{0.01}  & 25.43 & 27.22 & 50.48 & 59.86 \\
& DAG~\cite{xie2017adversarial} & 36.54 & 39.01 & 35.98 & 51.59 & 60.19 \\
& NI~\cite{lin2019nesterov} &1.55  & 16.65 & 18.26 & 45.76 & 49.89 \\
& DI~\cite{xie2019improving} & 2.32  & 19.87 & 23.61 & 52.63 & 55.32 \\
& TI~\cite{dong2019evading} &1.48  & 31.93 & 35.45 & 52.77 & 59.56 \\
& FSPGD (Ours) & 1.27  & \textbf{6.09}  & \textbf{3.78 } & \textbf{40.74} & \textbf{47.30} \\

\hline
\hline
\multirow{3}*{Source Models} & \multirow{2}*{Attack Method} & Source & PSP & DV3 & Segformer & Maskformer \\
& & Model & Res50 & Res50 & MiT-B0 & Swin-S \\
\cline{2-7}
& Clean Images & 65.65 / 67.16 & 64.62 & 65.90 & 60.58 & 68.24\\
\hline
\multirow{7}*{PSP} & PGD~\cite{mkadry2017towards} &1.80  & 9.71  & 12.80 & 48.83 & 59.57 \\
\multirow{7}*{Res101} & SegPGD~\cite{gu2022segpgd}&0.90  & 10.64 & 12.85 & 60.41 & 59.48 \\
& CosPGD~\cite{agnihotri2024cospgd} & \textbf{0.02}  & 14.02 & 16.41 & 50.75 & 61.01 \\
& DAG~\cite{xie2017adversarial}  & 35.74 & 23.56 & 33.92 & 51.65 & 61.42 \\
& NI~\cite{lin2019nesterov} &1.65  & 8.35  & 10.01 & 42.51 & 46.90 \\
& DI~\cite{xie2019improving} &2.18  & 16.94 & 19.39 & 50.57 & 53.31 \\
& TI~\cite{dong2019evading} & 1.73  & 25.15 & 29.84 & 50.95 & 57.30 \\
& FSPGD (Ours) & 2.29  & \textbf{5.96}  & \textbf{7.42}  & \textbf{36.63} & \textbf{36.91} \\

\hline
\multirow{7}*{DV3} & PGD~\cite{mkadry2017towards} &1.74  & 15.20 & 16.54 & 49.92 & 60.50 \\
\multirow{7}*{Res101} & SegPGD~\cite{gu2022segpgd} &0.63  & 17.29 & 18.04 & 50.18 & 60.11 \\
& CosPGD~\cite{agnihotri2024cospgd} &\textbf{0.01}  & 18.83 & 19.60 & 50.44 & 59.91 \\
& DAG~\cite{xie2017adversarial} &36.68 & 26.70 & 36.68 & 52.25 & 61.29 \\
& NI~\cite{lin2019nesterov} & 1.94  & 14.15 & 14.91 & 44.14 & 48.74 \\
& DI~\cite{xie2019improving} & 3.99  & 22.41 & 23.87 & 50.91 & 53.96 \\
& TI~\cite{dong2019evading} & 2.63  & 29.58 & 32.17 & 51.90 & 57.19 \\
& FSPGD (Ours) & 2.03  & \textbf{2.48}  &\textbf{ 3.25 } & \textbf{39.82 }& \textbf{47.04}\\
\Xhline{3\arrayrulewidth}

\end{tabularx}
\end{center}
\label{sup_table2}
\end{table}

\clearpage
% -----------------------------------------------------------------------

\section{Additional Examples for Qualitative Evaluation}
\label{sec: C}

\begin{figure}[htbp]
\centering
\includegraphics[width=0.80\linewidth]{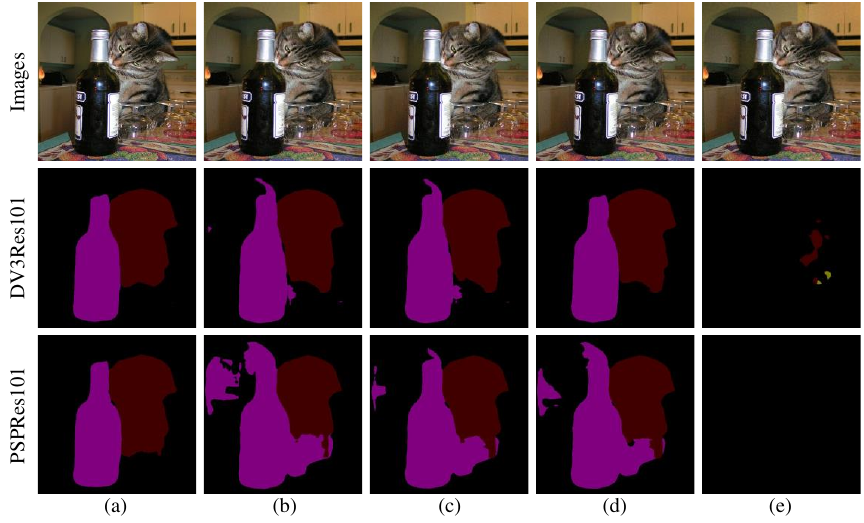}
\caption{Visualization of clean image, attacked images, and output predictions on Pascal VOC 2012. Deeplabv3-Res50 is used as the source model and Deeplabv3-Res101 (second row), and PSPNet-Res101 (third row) are used as target models. (a) Clean image, (b) PGD~\cite{mkadry2017towards}, (c) SegPGD~\cite{gu2022segpgd}, (d) CosPGD~\cite{agnihotri2024cospgd}, (e) FSPGD (Ours).}
\label{fig:figs5}
\end{figure}

\begin{figure}[htbp]
\centering
\includegraphics[width=0.80\linewidth]{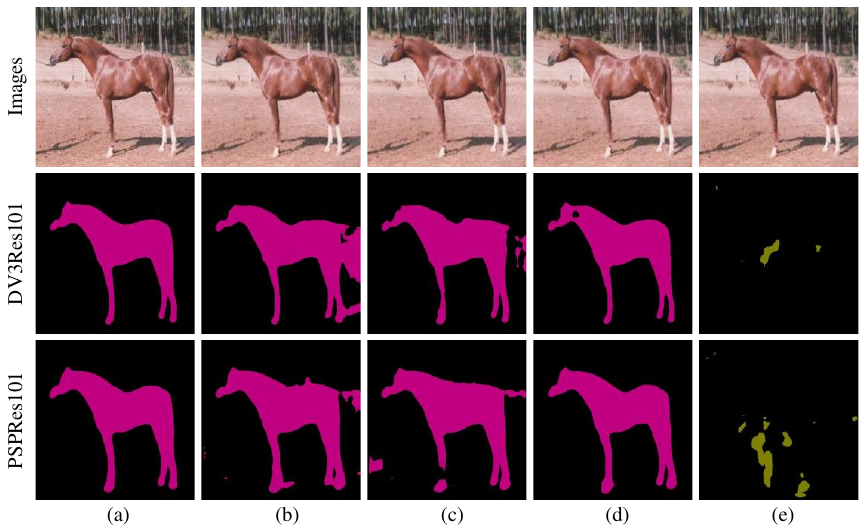}
\caption{Visualization of clean image, attacked images, and output predictions on Pascal VOC 2012. Deeplabv3-Res50 is used as the source model and Deeplabv3-Res101 (second row), and PSPNet-Res101 (third row) are used as target models. are used as target models. (a) Clean image, (b) PGD~\cite{mkadry2017towards}, (c) SegPGD~\cite{gu2022segpgd}, (d) CosPGD~\cite{agnihotri2024cospgd}, (e) FSPGD (Ours).}
\label{fig:figs6}
\end{figure}

\begin{figure}[htbp]
\centering
\includegraphics[width=0.65\linewidth]{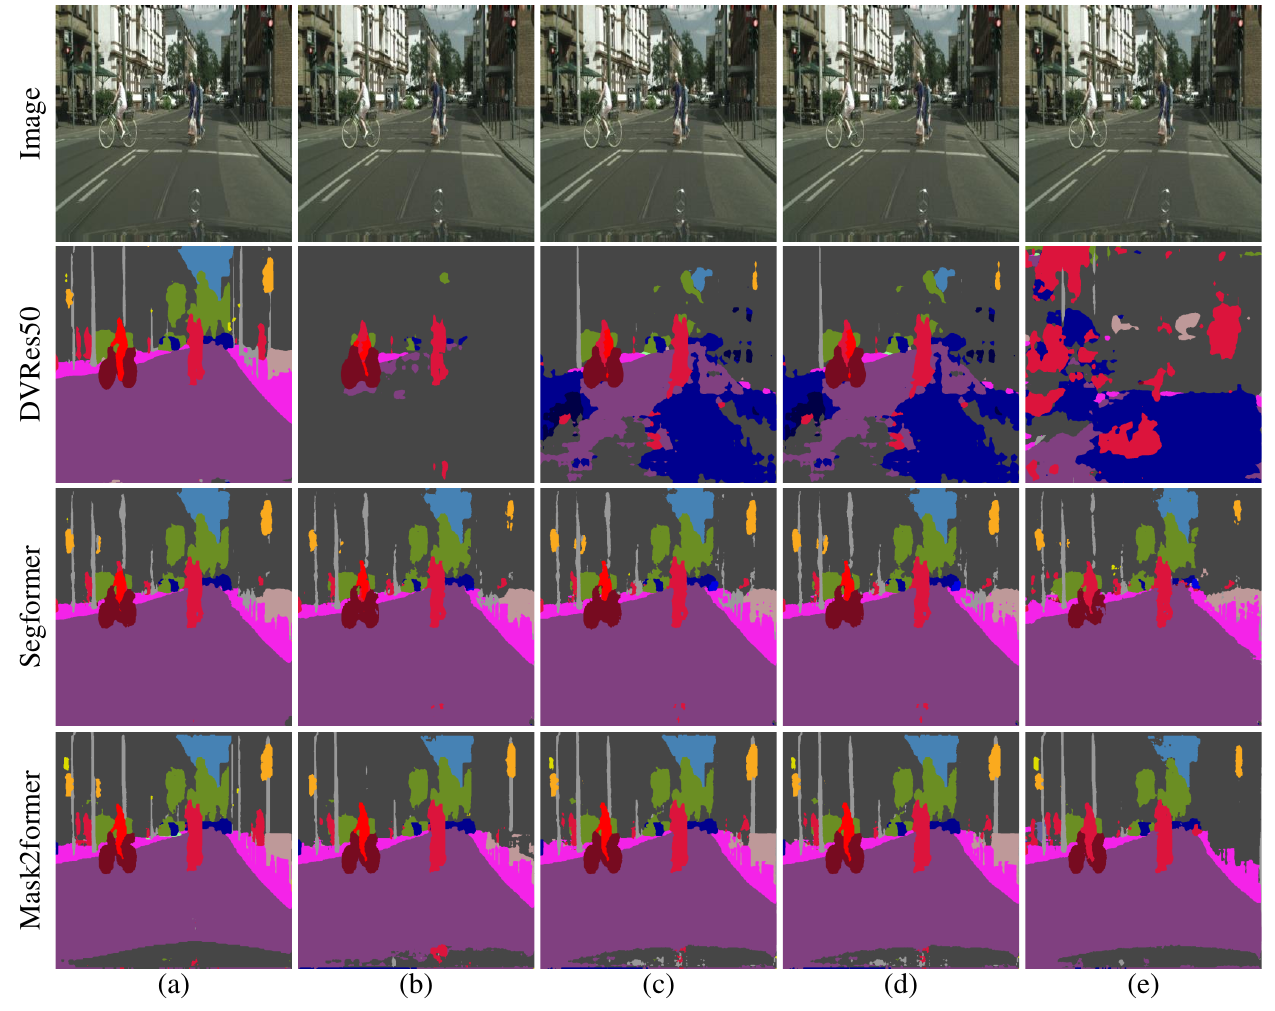}
\caption{Visualization of clean image, attacked images, and output predictions on Cityscapes. Deeplabv3-Res101 is used as the source model and Deeplabv3-Res50 (second row), Segformer-MiT B0 (third row), and Mask2former-SwinS (fourth row) are used as target models. (a) Clean image, (b) PGD~\cite{mkadry2017towards}, (c) SegPGD~\cite{gu2022segpgd}, (d) CosPGD~\cite{agnihotri2024cospgd}, (e) FSPGD (Ours).}
\label{fig:figs7}
\end{figure}

\begin{figure}[htbp]
\centering
\includegraphics[width=0.65\linewidth]{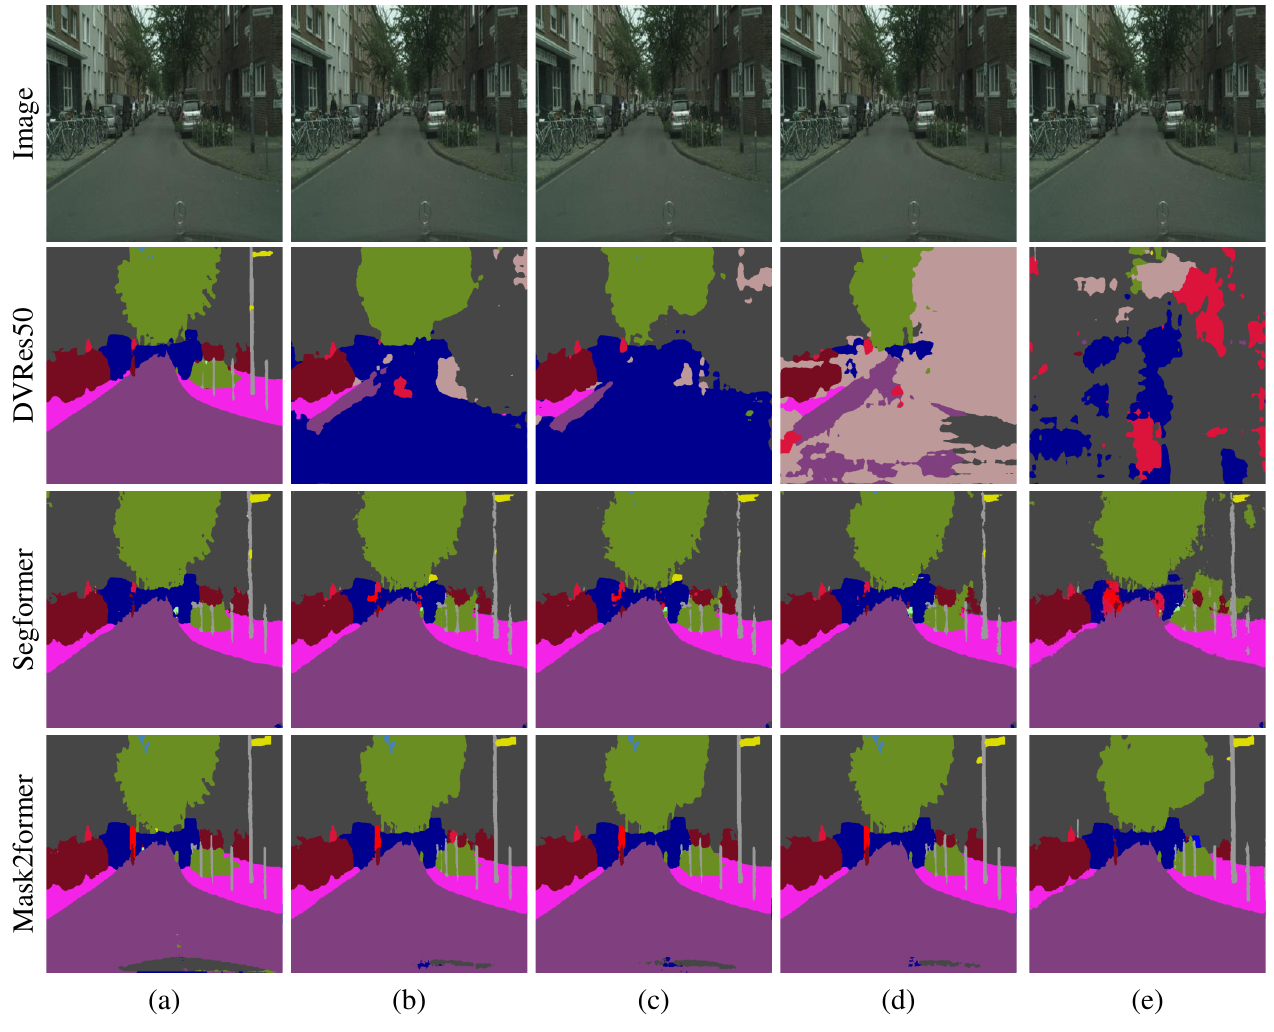}
\caption{Visualization of clean image, attacked images, and output predictions on Cityscapes.  Deeplabv3-Res101 is used as the source model and Deeplabv3-Res50 (second row), Segformer-MiT B0 (third row), and Mask2former-SwinS (fourth row) are used as target models. (a) Clean image, (b) PGD~\cite{mkadry2017towards}, (c) SegPGD~\cite{gu2022segpgd}, (d) CosPGD~\cite{agnihotri2024cospgd}, (e) FSPGD (Ours).}
\label{fig:figs8}
\end{figure}

\FloatBarrier
\newpage
\clearpage

%  % ade vis add 
% \begin{figure}[htbp]
% \centering
% \includegraphics[width=0.60\linewidth]{ade_vis1.pdf}
% \caption{Visualization of clean image, attacked images, and output predictions on ADE20K.  Segformer MiT B0 is used as the source model and Mask2former Swin-S (second row), Segformer-MiT B5 (third row), and Mask2former Swin-L (fourth row) are used as target models. (a) Clean image, (b) PGD~\cite{mkadry2017towards}, (c) SegPGD~\cite{gu2022segpgd}, (d) CosPGD~\cite{agnihotri2024cospgd}, (e) FSPGD (Ours).}
% \label{fig:figs9}
% \end{figure}

% \begin{figure}[htbp]
% \centering
% \includegraphics[width=0.60\linewidth]{ade_vis2.pdf}
% \caption{Visualization of clean image, attacked images, and output predictions on ADE20K.  Segformer MiT B0 is used as the source model and Mask2former Swin-S (second row), Segformer-MiT B5 (third row), and Mask2former Swin-L (fourth row) are used as target models. (a) Clean image, (b) PGD~\cite{mkadry2017towards}, (c) SegPGD~\cite{gu2022segpgd}, (d) CosPGD~\cite{agnihotri2024cospgd}, (e) FSPGD (Ours).}
% \label{fig:figs10}
% \end{figure}

% -----------------------------------------------------------------------
\section{Detailed Experimental Results for Ablation Studies}
\label{sec: D}
This section presents the quantified experimental results in ablation studies discussed in  Sec.~\ref{sec4.3:Ablation} and provides a more detailed explanation of these results. Additionally, it elaborates on ablation study findings that were not included in the main text due to space constraints.

\subsection{Performance comparison based on \texorpdfstring{$\tau$}{tau} value}
The proposed method includes a user-defined parameter, $\tau$, which is used to build the mask $\textrm{M}_B$. Since the $\tau$ value affects the attack performance, we conducted extensive experiments to compare the results. As shown in Table~\ref{sup_table4} and Table~\ref{sup_table5}, the attack performance varies slightly depending on the $\tau$ value. Notably, although performance fluctuates with different $\tau$ values, it consistently outperforms conventional techniques shown in Table~\ref{table1} and~\ref{table2} in main paper. We calculated the average performance for each  $\tau$ value and selected cos($\pi/3$) as the optimal value, as it achieved the highest average performance.

\begin{table*}[htbp]
\caption{Attack performance comparison in Pascal VOC 2012 dataset across different $\tau$ values. We measured mIoU scores and bold numbers indicate the best performance for each experimental setup.}
\begin{center}
% \renewcommand{\arraystretch}{1.15}

% \begin{tabular}{c | c | c  c  c  c}
\begin{tabularx}{\textwidth}{c|c|>{\centering\arraybackslash}X >{\centering\arraybackslash}X >{\centering\arraybackslash}X >{\centering\arraybackslash}X}
\Xhline{3\arrayrulewidth}
\multirow{2}*{Source Models} & \multirow{2}*{$\tau$} & \multicolumn{4}{c}{Target Models } \\
\cline{3-6}
&&{Source Model} & PSPRes101 & DVRes101 & FCNVGG16\\ 
\hline
\multirow{3}*{PSPRes50} & $\pi / 6$ & \textbf{3.37} & 28.49 & 22.05 & 21.39 \\
& $\pi / 4$ & 3.40 & 24.53 & 17.92 & 20.44 \\
& $\pi / 3$ & 3.39 & \textbf{22.24} & \textbf{16.84} & \textbf{19.75} \\
% & $\pi / 2$ & 3.87 & 43.03 & 37.51 & 27.49 \\
\hline
\multirow{3}*{DV3Res50} & $\pi / 6$ & 3.46 & 27.52 & 22.01 & 20.98 \\
& $\pi / 4$ & 3.45 & 23.85 & 17.77 & 20.16 \\
& $\pi / 3$ & \textbf{3.44} & \textbf{21.89} & \textbf{16.57} & \textbf{19.36} \\
% & $\pi / 2$ & 3.86 & 41.02 & 36.54 & 26.93 \\
\hline
\hline
\multirow{2}*{Source Models} & \multirow{2}*{$\tau$} & \multicolumn{4}{c}{Target Models } \\
\cline{3-6}
&&{Source Model} & PSPRes50 & DVRes50 & FCNVGG16\\ 
\hline
\multirow{3}*{PSPRes101} & $\pi / 6$ & 3.01 & 20.89 & 20.30 & 24.10 \\
& $\pi / 4$  &  3.04 & \textbf{11.77} &\textbf{12.30} & 21.55 \\
& $\pi / 3$ &  \textbf{ 2.99} & 12.48 & 13.54 & \textbf{21.30} \\
% & $\pi / 2$ & 3.59 & 26.30 & 28.07 & 27.81 \\
\hline
\multirow{3}*{DV3Res101} 
& $\pi / 6$ & 3.29 & 21.43 & 20.69 & 24.52 \\
& $\pi / 4$ & \textbf{3.25} & \textbf{11.37} & \textbf{11.95} & 21.57 \\
& $\pi / 3$ & 3.28 & 11.42 & 13.45 & \textbf{21.49 }\\
% & $\pi / 2$& 3.58 & 26.48 & 29.02 & 28.80 \\
\hline
\Xhline{3\arrayrulewidth}
\end{tabularx}
\end{center}
\label{sup_table4}
\end{table*}

\begin{table*}[htbp]
\caption{Attack performance comparison in Cityscapes dataset across different $\tau$ values. We measured mIoU scores and bold numbers indicate the best performance for each experimental setup.}
\begin{center}
\begin{tabularx}{\textwidth}{c|c|>{\centering\arraybackslash}X >{\centering\arraybackslash}X >{\centering\arraybackslash}X >{\centering\arraybackslash}X >{\centering\arraybackslash}X >{\centering\arraybackslash}X}
\Xhline{3\arrayrulewidth}
& & \multicolumn{6}{c}{Target Models (mIoU$\downarrow$)}\\
\hline
\multirow{2}*{Source Models} & \multirow{2}*{$\tau$} & Source & PSP & DV3 & PSP & DV3 & Mask2former \\
& & Model & Res50 & Res50 & Res101 & Res101 & Swin-S \\
\hline
\multirow{2}*{Segformer} & $\pi / 6$  & 1.70 & 9.98 &16.38&25.98&25.08& 43.74 \\
\multirow{2}*{MiT-B0} & $\pi / 4$ &  1.36 &11.19&16.59&24.76 & 24.81 &42.97 \\
& $\pi / 3$  & 1.33& 10.09&14.57& 21.16 & 22.06 &\textbf{39.92} \\
% & $\pi / 2$  & \textbf{1.28 } & \textbf{9.59}& \textbf{13.49} &\textbf{20.87} & \textbf{20.75} & 40.55 \\
\hline
\hline
\multirow{2}*{Source Models} & \multirow{2}*{$\tau$} & Source & PSP & DV3 & PSP & DV3 & Segformer \\
& & Model & Res50 & Res50 & Res101 & Res101 & MiT-B0 \\
\hline
\multirow{2}*{Mask2former} & $\pi / 6$ & 4.15 &16.83 &20.47&26.13 & 28.58 &38.84 \\
\multirow{2}*{Swin-S} & $\pi / 4$ &2.94 & 16.62&19.61&24.64 & 26.78 & 37.80 \\
& $\pi / 3$ &\textbf{2.20 } & \textbf{15.57} &  18.00&24.29 & 25.96 & 36.87 \\
% & $\pi / 2$ &2.94 & 15.90 & \textbf{17.82} & \textbf{23.66} & \textbf{25.24} & \textbf{36.35} \\

\Xhline{3\arrayrulewidth}

\end{tabularx}
\end{center}
\label{sup_table5}
\end{table*}

\clearpage

% -----------------------------------------------------------------------
\newpage
% lambda
\subsection{Performance comparison based on \texorpdfstring{$\lambda$}{lambda} value}
The proposed loss function consists of two loss terms, $L_{ex}$ and $L_{in}$. Here, we provide a detailed numerical explanation of the experimental results, along with additional results for loss term combinations. Table~\ref{sup_table4} summarizes the experimental results on the Pascal VOC 2012 and Cityscapes dataset. As shown in Table~\ref{sup_table6} and \ref{sup_table7}, the performance of the proposed method varies depending on how the two loss terms are combined. As discussed in the main text, simply adding the two loss terms can result in a compromise, leading to lower performance compared to using $L_{ex}$ alone.  To investigate this performance degradation, we conducted experiments with different ratios, such as $L_{ex} + 0.5L_{in}$ and $L_{ex} + 0.1L_{in}$. The results, as summarized in the Table~\ref{sup_table6} and \ref{sup_table7}, show that performance varies depending on the source model; for instance, when PSPNet-Res50 is the source model, performance was lower compared to using $L_{ex}$ alone, but when DeepLabv3-Res50 was used, performance improved. To address this issue of performance variation across source models, we proposed a dynamic $\lambda_{t}$ that adjusts with \textit{t}, and this method demonstrated the best performance overall.

\begin{table}[htbp]
\caption{Attack performance comparison across different loss combinations. We measured mIoU scores and bold numbers indicate the best performance for each experimental setup.}
\begin{center}

\begin{tabular}{c | c | c  c  c  c}
\Xhline{3\arrayrulewidth}
& & \multicolumn{4}{c}{Target Models } \\
\hline
Source Models&$\lambda$ &{Source Model} & PSPRes101 & DVRes101 & FCNVGG16\\ 
\hline

\multirow{6}*{PSPRes50} 
& $L_{ex}$ & \textbf{3.37} & 24.81 & 18.13 & 20.01 \\
& $L_{in}$ & 4.06 & 60.96 & 61.92 & 37.09 \\
& $L_{ex} + L_{in}$ & 3.40 & 25.78 & 19.11 & 20.98 \\
& $L_{ex} + 0.5L_{in}$ & 3.41 & 25.07 & 18.51 & 20.44 \\
& $L_{ex} + 0.1L_{in}$ & 3.37 & 24.93 & 18.16 & 20.13 \\
& $\lambda_t L_{ex} + (1-\lambda_t)L_{in}$ & 3.39 & \textbf{22.24} & \textbf{16.84} & \textbf{19.75} \\
\hline

\multirow{6}*{DV3Res50} 
& $L_{ex}$  & 3.47 & 25.19 & 18.93 & 19.78 \\
& $L_{in}$  & 4.01 & 58.42 & 58.87 & 36.90 \\
& $L_{ex} + L_{in}$ & 3.45 & 24.69 & 19.35 & 20.54 \\
& $L_{ex} + 0.5L_{in}$ & 3.45 & 24.76 & 18.73 & 20.08 \\
& $L_{ex} + 0.1L_{in}$ & 3.45 & 24.86 & 18.64 & 19.75 \\
& $\lambda_t L_{ex} + (1-\lambda_t)L_{in}$ & \textbf{3.44} & \textbf{21.89} & \textbf{16.57} & \textbf{19.36} \\
\hline\hline
Source Models  &$\lambda$  &  Source Model & PSPRes50 & DVRes50 & FCNVGG16 \\ 
\hline
\multirow{6}*{PSPRes101} 
& $L_{ex}$ & 3.13 & 14.36 & 14.68 & 21.03 \\
& $L_{in}$ & 4.75 & 45.67 & 48.64 & 37.59 \\
& $L_{ex} + L_{in}$ & 3.04 & 12.97 & 14.57 & 21.41 \\
& $L_{ex} + 0.5L_{in}$ & 3.06 & 13.17 & 14.22 & 21.08\\
& $L_{ex} + 0.1L_{in}$ & 3.12 & 13.83 & 14.48 & \textbf{21.02} \\
& $\lambda_t L_{ex} + (1-\lambda_t)L_{in}$ &  \textbf{2.99} & \textbf{12.48} & \textbf{13.54} & 21.30 \\

\hline
\multirow{6}*{DV3Res101} 
& $L_{ex}$ & 3.32 & 12.60 & \textbf{13.44} & \textbf{20.57} \\
& $L_{in}$ & 17.54 & 65.77 & 66.57 & 39.99 \\
& $L_{ex} + L_{in}$ & 3.71 & 32.42 & 30.21 & 23.37 \\
& $L_{ex} + 0.5L_{in}$ & 3.61 & 29.84 & 27.75 & 22.20 \\
& $L_{ex} + 0.1L_{in}$ & 3.57 & 27.86 & 25.17 & 21.12 \\
& $\lambda_t L_{ex} + (1-\lambda_t)L_{in}$ &\textbf{3.28} & \textbf{11.42} & 13.45 & 21.49 \\
\hline
\Xhline{3\arrayrulewidth}
\end{tabular}
\end{center}
\label{sup_table6}
\end{table}

\begin{table}[htbp]
\caption{Attack performance comparison across different loss combinations. We measured mIoU scores and bold numbers indicate the best performance for each experimental setup.}
\begin{center}

\begin{tabular}{c | c | c  c  c  c  cc}
\Xhline{3\arrayrulewidth}
& & \multicolumn{5}{c}{Target Models} \\
\hline
\multirow{2}*{Source Models}  &\multirow{2}*{$\lambda$} &Source & PSP & DV & PSP & DV &  Mask2former\\ 
& &Model &  Res50 & Res50 &  Res101 & Res101 & Swin-S\\ 
\hline
\multirow{5}*{Segformer} 
& $L_{ex}$ &   60.20 &  55.94 &  60.08 &  60.20 &  64.11 &  64.62 \\
\multirow{5}*{MiT-B0} & $L_{in}$& 21.73 & 30.56 & 28.59 & 36.75 & 37.91 & 47.93 \\
& $L_{ex} + L_{in}$ & 56.43 & 52.85 & 56.40 & 57.59 & 60.04 & 63.53 \\
& $L_{ex} + 0.5L_{in}$& 58.46 & 54.55 & 58.78 & 59.34 & 62.27 & 64.17 \\
& $L_{ex} + 0.1L_{in}$& 59.92 & 55.61 & 59.80 & 60.47 & 63.78 & 64.49 \\
& $\lambda_t L_{ex} + (1-\lambda_t)L_{in}$ &\textbf{ 1.33}  & \textbf{10.09} &\textbf{ 14.57 }& \textbf{21.16} & \textbf{22.06} & \textbf{39.92} \\
\hline
\hline
\multirow{2}*{Source Models}  &\multirow{2}*{$\lambda$} &Source & PSP & DV & PSP & DV &  Segformer\\ 
& &Model &  Res50 & Res50 &  Res101 & Res101 & MiT-B0\\ 
\hline
\multirow{5}*{Maskformer} 
& $L_{ex}$ & 67.05 & 58.61 & 61.84 & 61.77 & 64.21 &58.58\\
\multirow{5}*{Swin-S} & $L_{in}$ &24.05 & 44.91 & 44.76 & 44.77 & 50.27 & 51.84 \\
& $L_{ex} + L_{in}$ & 64.58 & 55.94 & 59.34 & 59.00 & 62.06 & 57.42 \\
& $L_{ex} + 0.5L_{in}$ &65.99 & 57.40 & 60.67 & 60.79 & 63.28 & 57.97 \\
& $L_{ex} + 0.1L_{in}$ & 67.43 & 58.38 & 61.59 & 61.87 & 64.38 & 58.52 \\
& $\lambda_t L_{ex} + (1-\lambda_t)L_{in}$ &\textbf{2.20}  & \textbf{15.57} &  \textbf{18.00}&\textbf{24.29} & \textbf{25.96} & \textbf{36.87} \\
\Xhline{3\arrayrulewidth}

\end{tabular}
\end{center}
\label{sup_table7}
\end{table}
\FloatBarrier
\newpage
\clearpage

% -----------------------------------------------------------------------

% layer
\subsection{Performance comparison based on layer location}
Unlike conventional methods, the proposed method performs attacks by leveraging intermediate-layer features, making it the first approach to introduce intermediate-layer attacks in the field of semantic segmentation. As such, unlike intermediate-layer attack methods in image classification, there is no prior research on which layer is optimal for attacks in semantic segmentation. To address this, we conducted extensive experiments by attacking various layers of the encoder and summarized the results. Tables~\ref{sup_table8}, ~\ref{sup_table9}, and ~\ref{sup_table10} present the intermediate-layer attack performance for ResNet50, ResNet101 encoders, and transformer encoders, respectively. Attacking the later layers of the encoder (\ie, layer 4\_2) results in strong performance on the source model but poor performance on the target models. In contrast, attacking the middle layers demonstrates reasonable attack performance on the source model while also achieving high transferability. Therefore, as the proposed method aims to enhance transferability, we chose to attack the middle layers.

\begin{table*}[htbp]
\caption{Attack performance results on source models using the ResNet50 encoder across different attack layers, evaluated on the Pascal VOC 2012 dataset. We measured mIoU scores and bold numbers indicate the best performance for each experimental setup.}
\begin{center}

\begin{tabular}{c | c | c  c  c  c}

\Xhline{3\arrayrulewidth}

\multirow{2}*{Source Models} & \multirow{2}*{Layer name} & \multicolumn{4}{c}{Target Models } \\
\cline{3-6}
&&{Source Model} & PSPRes101 & DVRes101 & FCNVGG16\\

\hline

\multirow{10}*{PSPRes50} 
& 2\_1  
& 11.42 & 50.11 & 50.89 & 22.95 \\
& 2\_2
& 5.75 & 44.51 & 43.05 & 23.90 \\
& 2\_3
& 5.87 & 45.12 & 41.42 & 25.22 \\
& 3\_1
& 3.45 & 26.42 & 20.49 & 19.34 \\
& 3\_2
& 3.39 & \textbf{22.24} & \textbf{16.84} & \textbf{19.75} \\
& 3\_3
& 3.37 & 22.39 & 16.84 & 21.36 \\
& 3\_4
& 3.28 & 24.35 & 18.74 & 22.30 \\
& 3\_5
& 3.24 & 26.04 & 19.83 & 24.03 \\
& 4\_1
& 2.82 & 52.72 & 51.89 & 34.52 \\
& 4\_2
& \textbf{1.92} & 69.88 & 72.03 & 42.22 \\
\hline

\multirow{10}*{DV3Res50} 
& 2\_1  
& 8.11 & 48.15 & 47.67 & 22.10 \\
& 2\_2
& 4.45 & 41.36 & 38.61 & 22.42 \\
& 2\_3
& 4.74 & 41.45 & 38.47 & 23.86 \\
& 3\_1
& 3.47 & 26.37 & 20.33 & \textbf{18.81} \\
& 3\_2
& 3.44 & \textbf{21.89} & \textbf{16.57} & 19.36 \\
& 3\_3
& 3.39 & 22.19 & 17.47 & 20.93 \\
& 3\_4
& 3.35 & 24.19 & 19.22 & 22.22 \\
& 3\_5
& 3.26 & 24.99 & 19.52 & 23.77 \\
& 4\_1
& 2.38 & 50.66 & 51.72 & 34.40 \\
& 4\_2
& \textbf{2.36} & 67.71 & 69.74 & 41.08 \\

\Xhline{3\arrayrulewidth}

\end{tabular}
\end{center}
\label{sup_table8}
\end{table*}

\begin{table}[htbp]
\caption{Attack performance results on source models using the ResNet101 encoder across different attack layers, evaluated on the Pascal VOC 2012 dataset. We measured mIoU scores and bold numbers indicate the best performance for each experimental setup.}
\begin{center}

\begin{tabular}{c | c | c  c  c  c}

\Xhline{3\arrayrulewidth}

\multirow{2}*{Source Models} & \multirow{2}*{Layer name} & \multicolumn{4}{c}{Target Models } \\
\cline{3-6}
&&{Source Model} & PSPRes50 & DVRes50 & FCNVGG16\\

\hline
\multirow{12}*{PSPRes101} 

& 2\_1  
& 17.14 & 50.60 & 44.57 & 24.51 \\
& 2\_2
& 5.84 & 37.81 & 33.03 & 22.56 \\
& 2\_3
& 5.41 & 38.71 & 33.99 & 23.97 \\
& 3\_1
& 3.11 & 31.59 & 29.55 & 22.23 \\
& 3\_2
& 3.46 & 34.19 & 30.77 & 23.29 \\
& 3\_5
& 3.44 & 17.41 & 17.12 & \textbf{19.48} \\
& 3\_10
& 2.99 & \textbf{12.48} & \textbf{13.54} & 21.30 \\
& 3\_15
& 3.05 & 18.20 & 17.82 & 24.12 \\
& 3\_20
& 3.05 & 36.45 & 35.41 & 31.44 \\
& 3\_22
& 2.93 & 40.76 & 41.55 & 34.30 \\
& 4\_1
& 3.11 & 56.98 & 55.85 & 37.44 \\
& 4\_2
& \textbf{2.78} & 65.26 & 64.50 & 41.44 \\
\hline

\multirow{12}*{DV3Res101} 
& 2\_1  
& 17.78 & 51.02 & 44.56 & 24.57 \\
& 2\_2
& 7.40 & 37.30 & 32.94 & 22.94 \\
& 2\_3
& 6.38 & 41.47 & 34.65 & 24.49 \\
& 3\_1
& 3.36 & 32.32 & 31.56 & 22.26 \\
& 3\_2
& 3.57 & 33.69 & 32.74 & 23.79 \\
& 3\_5
& 3.46 & 17.33 & 17.68 & \textbf{19.85} \\
& 3\_10
& 3.28 & \textbf{11.42} & \textbf{13.45} & 21.49 \\
& 3\_15
& 3.35 & 18.55 & 19.01 & 25.20 \\
& 3\_20
& 3.38 & 38.31 & 39.72 & 33.36 \\
& 3\_22
& 3.25 & 43.07 & 45.80 & 35.58 \\
& 4\_1
& 3.17 & 57.74 & 56.16 & 38.35 \\
& 4\_2
& \textbf{1.49} & 63.18 & 62.93 & 40.99 \\
\Xhline{3\arrayrulewidth}

\end{tabular}
\end{center}
\label{sup_table9}
\end{table}

\begin{table}[htbp]
\caption{Attack performance results on source models using the transformer encoder across different attack layers, evaluated on the Cityscapes dataset. We measured mIoU scores and bold numbers indicate the best performance for each experimental setup.}
\begin{center}

\setlength{\tabcolsep}{2pt}

% \begin{tabular}{c | c | c c  c  c  c c c}
\begin{tabularx}{\textwidth}{c|c|>{\centering\arraybackslash}X >{\centering\arraybackslash}X >{\centering\arraybackslash}X >{\centering\arraybackslash}X >{\centering\arraybackslash}X >{\centering\arraybackslash}X >{\centering\arraybackslash}X}

\Xhline{3\arrayrulewidth}

 && \multicolumn{6}{c}{Target Models } \\
\hline

Source & \multirow{2}*{Layer name}& Source &PSP & DV3 & PSP & DV3 & Mask2former\\
Models&&Model& Res50 & Res50& Res101 & Res101 & Swin-S\\

\hline
\multirow{11}*{Segformer} 
& patch\_embeddings-0 &43.55 & 25.45 & 27.83 & 30.83 & 33.77 & 51.55 \\
\multirow{11}*{MiT-B0} & patch\_embeddings-1 & 2.54  & 10.88 & 17.94 & 23.39 & 25.40 & 43.25 \\
& patch\_embeddings-2 &1.53  & 13.56 & 17.04 & 27.39 & 25.47 & 42.05 \\
& patch\_embeddings-3 &0.67  & 13.97 & 15.49 & 25.53 & 22.75 & 44.06 \\
& block-0-0 &22.11 & 16.02 & 23.01 & 26.31 & 28.99 & 51.51 \\
& block-0-1 &15.28 & 12.53 & 18.58 & 24.94 & 28.53 & 46.98 \\
& block-1-0 & 1.33  & 10.09 & 14.57 & \textbf{21.16} & 22.06 & \textbf{39.92} \\
& block-1-1 & 1.16  & \textbf{9.02}  & \textbf{13.11} & 24.03 & 21.58 & 43.41 \\
& block-2-0 & 1.01  & 12.72 & 13.80 & 22.98 & \textbf{20.18} & 40.12 \\
& block-2-1 &0.86  & 11.85 & 13.94 & 23.82 & 21.94 & 41.06 \\
& block-3-0 &0.33  & 17.79 & 18.56 & 27.58 & 25.99 & 45.51 \\
& block-3-1 & \textbf{0.16}  & 24.99 & 25.54 & 33.59 & 34.81 & 50.41 \\

\hline
\hline

Source & \multirow{2}*{Layer name}& Source &PSP & DV3 & PSP & DV3 & Segformer\\
Models&&Model& Res50 & Res50& Res101 & Res101 & MiT-B0\\

\hline
\multirow{8}*{Mask2former} 
& embeddings &57.96 & 27.09 & 40.40 & 34.54 & 44.27 & 53.06 \\
\multirow{8}*{Swin-S} & layers-0-blocks-0 &48.77 & 23.98 & 38.13 & 29.91 & 42.71 & 50.91 \\

& layers-0-blocks-1 &37.73 & 16.41 & 33.17 & 24.86 & 36.57 & 46.63 \\
& layers-1-blocks-0 &33.11 & 19.11 & 25.37 & 23.72 & 29.57 & 44.34 \\
& layers-1-blocks-1 &17.77 & \textbf{13.65} & 25.81 & 19.64 & 28.03 & 41.63 \\
& layers-2-blocks-0 &2.20  & 15.57 & \textbf{24.29} & \textbf{18.00 }& \textbf{25.96} & \textbf{36.87} \\
& layers-2-blocks-17&\textbf{0.79}  & 30.47 & 36.66 & 31.20 & 38.85 & 45.15 \\
& layers-3-blocks-0 &1.11  & 31.94 & 38.83 & 34.20 & 41.06 & 45.86 \\
& layers-3-blocks-1 &1.41  & 33.83 & 40.14 & 36.43 & 43.11 & 46.49 \\

\Xhline{3\arrayrulewidth}

\end{tabularx}
\end{center}
\label{sup_table10}
\end{table}

\FloatBarrier
\newpage
\clearpage
